# Supplementary material for: Learning Domain Invariant Representations for Generalizable Person Re-Identification
Source: arXiv:2103.15890 source file (2022-12-17)
Supplement: Supplementary file 1 [file appendix.tex]

%\appendix

% Remove page # from the first page of camera-ready.
\subsection{Derivation of the Interventional Distribution $P(Y|do(S))$ for the Proposed Causal Graph}\label{proof:intervention}
The following proof is similar to~\cite{yue2020interventional} with three rules of \textit{do}-calculus~\cite{pearl1995causal}: Insertion/deletion of observations, Action/observation exchange and Insertion/deletion of actions.

%Given a causal directed acyclic graph $\mathcal{G}$, denote $X,Y,Z$ and $W$ be arbitrary disjoint sets of nodes. We use $\mathcal{G}_{\overline{X}}$ to denote the manipulated graph where all incoming arrows to node $X$ are deleted. Similarly $\mathcal{G}_{\underline{X}}$ represents the graph where outgoing arrows from node $X$ are deleted. Lower case $x,y,z$ and $w$ denote specific values taken by each set of nodes: $X=x,Y=y,Z=z$ and $W=w$. For any interventional distribution compatible with $\mathcal{G}$, we have the following three rules:

\begin{comment}
\noindent\textbf{Rule 1} Insertion/deletion of observations:
\begin{equation}
    P(y|do(x),z,w)=P(y|do(x),w), if(Y\Vbar Z|X,W)_{\mathcal{G}_{\overline{X}}}
\end{equation}

\noindent\textbf{Rule 2} Action/observation exchange:
\begin{equation}
\small
    P(y|do(x),do(z),w)=P(y|do(x),z,w), if(Y\Vbar Z|X,W)_{\mathcal{G}_{\overline{X}\underline{Z}}}
\end{equation}

\noindent\textbf{Rule 3} Insertion/deletion of actions:
\begin{equation}
\small
    P(y|do(x),do(z),w)=P(y|do(x),w), if(Y\Vbar Z|X,W)_{\mathcal{G}_{\overline{X}\overline{Z(W)}}},
\end{equation}
where $Z(W)$ is a set of nodes in $Z$ that are not ancestors of any $W$-node in $\mathcal{G}_{\overline{X}}$.
\end{comment}

In our causal formulation, the desired interventional distribution $P(Y|do(S=s))$ can be derived by:

\begin{equation}
\begin{aligned}
     P(Y|do(S))&=\sum_{v} P(Y|do(S=s),V=v)P(V=v|do(S=s))\\
     &=\sum_{v} P(Y|do(S=s),V=v)P(V=v)\\
     &=\sum_{v} P(Y|S=s,V=v)P(V=v),
\end{aligned}
\end{equation}
where line 1 follow the law of total probability; line 2 uses Rule 3 given $S\Vbar V$ in $\mathcal{G}_{\overline{X}}$; line 3 uses Rule 2 to change the intervention term to observation as $(Y\Vbar S|V)$ in $\mathcal{G}_{\underline{X}}$.

\subsection{Analysis of the Multi-Domain Disentangled Adversarial Neural Network (MDDAN)}
\label{app:max_ent}
Here we adapt from~\cite{Qi_2019_ICCV} and prove the Lemma 1 in the original manuscript. All the analyses are conducted in the shared ID-specific representation space. We first prove the following lemma.
%the proof is inspired by~\cite{Qi_2019_ICCV}. The difference is that, in~\cite{Qi_2019_ICCV}, they want to alleviate the discrepancy across all cameras between source domain and target domain, while we remove the discrepancy across multi source domains. 

\begin{lemma}
    When MDDAN is carried out and the uncertainty is maximized, given any ID-specific representation $\mathbf{s}^\tau$ of an image from domain $\mathcal{D}_\tau$, the conditional probability of any $\mathcal{D}_i$ given $\mathbf{s}^\tau$ will equal $1/K$, namely for any $i=1,...,K$, we have $p(\mathcal{D}_i|\mathbf{s}^\tau)=1/K$.
\end{lemma}~\label{lemma:UMS1}
\begin{proof}
    Here we slightly abuse the notation: omitting the domain classifier $\mathcal{C}_V$ and $ p(k|\mathbf{s}^\tau)$ is equivalent to $ p(\mathcal{D}_k|\mathbf{s}^\tau)$. MDDAN is defined as follows.
    \begin{equation}
        \begin{split}
        &\max -\sum_{k=1}^K p(k|\mathbf{s}^\tau)\log p(k|\mathbf{s}^{\tau}), \\
        &\text{ s.t.}~\sum_{k=1}^K{ p(k|\mathbf{s}^\tau)}=1;  p(k|\mathbf{s}^\tau)\geq0, \forall k.
        \end{split}
        \end{equation}

    Let $\mathcal{H}(p_k)=p_{k}\log p_{k}$, where $p_k=p(k|\mathbf{s}^\tau)$. We simplify the above optimization problem as
    \begin{equation}
    \min\sum_{k=1}^K\mathcal{H}(p_k), \text{ s.t.}~\sum_{k=1}^K{p_{k}}=1;p_{k}\geq0,\forall k,
    \end{equation}

    where $\mathcal{H}(p_{k})$ is convex as we have $\mathcal{I}''(p_k)=\frac{1}{p_k\ln2}>0$.
    The sum of convex functions $\sum_{k=1}^K{\mathcal{H}(p_k)}$ is also a convex function. Namely, this problem is a convex optimization problem. To prove the lemma, it is now equivalent to show that the minimum value of this convex optimization problem is obtained when $p_1=p_2=...=p_K=1/K$.
    
    We use the \textit{augmented Lagrangian method} to solve the problem, where the Lagrange function is defined as
    \begin{equation}
        L(p,\lambda)=\sum_{k=1}^K{p_k\log p_k}+\lambda(\sum_{k=1}^K{p_k}-1)).
    \end{equation}
    We take partial derivatives for each $p_k$ and get
    \begin{equation}
        \frac{\partial{L(p,\lambda)}}{\partial{p_k}}=\log{p_k}+\frac{1}{\ln2}+\lambda=0.
    \end{equation}
    Then we have $p_k=2^{-\lambda-1/\ln2}$. As $\sum_{k=1}^K{p_k}=1$, we have $K*2^{-\lambda-1/\ln2}=1$, and thus $p_k=1/K, i=1,2,...,K$.
    Since the local minimum of the convex function is the global minimum, when $p_1=p_2=...=p_K=1/K$, $\sum_{k=1}^K{\mathcal{H}(p_k)}$ achieves the minimum value, $\log \frac{1}{K}$.
    In other words, when MDDAN is carried out and achieves the maximum uncertainty, for all $i=1,...,K$, we have $p(\mathcal{D}_i|\mathbf{s}^\tau)=1/K$.
\end{proof}
Now we are ready to prove Lemma 1. we can calculate any domain $\mathcal{D}_i$'s conditional probability given $\mathbf{s}^\tau$, which is
\begin{equation}
    p(\mathcal{D}_i|\mathbf{s}^\tau)=\frac{p(\mathbf{s}^\tau|\mathcal{D}_i)p(\mathcal{D}_i)}{p_\tau(\mathbf{s}^\tau)}, \forall \mathbf{s}^\tau\in \mathcal{D}_\tau; i=1,...,K,
\label{equ:equal}
\end{equation}
where $p(\mathbf{s}^\tau|\mathcal{D}_i)$ denotes the conditional probability of $\mathbf{s}^\tau$ given domain information $\mathcal{D}_i$, $p_\tau(\mathbf{s}^\tau)$ denotes the probability function of the ID-specific representation in its domain $\mathcal{D}_{\tau}$, and $p(\mathcal{D}_i)$ is the priori probability of domain classes. Without generality, we set equal priori probability for each domain, namely $p(\mathcal{D}_i)=1/K$. Further, from the Lemma~\ref{lemma:UMS1} we know that, optimizing MDDAN leads to $p(\mathcal{D}_i|\mathbf{s}^\tau)=1/K$ for all $i=1,...,K$. Hence, \myref{equ:equal} becomes 

\begin{equation}
    \begin{split}
    &1/K=\frac{p(\mathbf{s}^\tau|\mathcal{D}_i)1/K}{p_\tau(\mathbf{s}^\tau)}, \forall \mathbf{s}^\tau\in \mathcal{D}_\tau; i=1,...,K,\\
    \Rightarrow &p(\mathbf{s}^\tau|\mathcal{D}_i)=p_\tau(\mathbf{s}^\tau), \forall \mathbf{s}^\tau\in \mathcal{D}_\tau; i=1,...,K,
    \end{split}
    \end{equation}
thus completes the proof.

\subsection{Understanding MDDAN by Information Theory}
\label{app:info}
Minimizing the mutual information between the ID-specific factors $S$ and the domain information $D$ is defined as

\begin{equation}
    \begin{aligned}
         \min \mathcal{I}(S,D)&=\min \mathcal{H}(D)-\mathcal{H}(D|S)\\
         &=\min -\mathcal{H}(D|S)\\
         &=\max \mathcal{H}(D|S)
    \end{aligned}
\end{equation}

The second line is derived since the entropy of domain distribution $\mathcal{H}(D)$ is not related to our optimization. Namely, our MDDAN is essentially minimizing the mutual information between the ID-specific factors and the domain information.
% \begin{table}[]
%     \centering
%     \begin{tabular}{c|ccc}
%     \hline
%     Collection & Dataset& IDs & Images  \\ \hline
%      \multirow{5}{*}{MS} & CUHK02& 1,816 & 7,264  \\ 
%                                          & CUHK03& 1,467 & 14,097  \\ 
%                                    & DukeMTMC-Re-Id & 1,812 & 36,411  \\ 
%                                          &Market-1501& 1,501 & 29,419  \\ 
%                                          &CUHK-SYSU& 11,934 & 34,547  \\ \hline\hline
%     \end{tabular}
%  \caption{Training Datasets Statistics. All the images in these datasets, regardless of their original train/test splits, are used for model training.}\label{tab:traindata}
%  \end{table}
 
%  \begin{table}[]
%     \centering
%     \begin{tabular}{c|c|c|c|c}
%     \hline
%     \multirow{2}{*}{Dataset} & \multicolumn{2}{c|}{ Probe} & \multicolumn{2}{c}{  Gallery} \\\cline{2-5} 
%      &            Pr. IDs&           Pr. Imgs&           Ga. IDs&    Ga. imgs       \\\hline
%                       PRID&           100& 100         &     649      &    649      \\
%                       GRID&           125& 125          &   1025        &    1,025      \\
%                       VIPeR&           316&   316    &    316     &    316    \\
%                       i-LIDS&           60&60          &          60 &    60     \\\hline\hline
%  \end{tabular}
%  \caption{Testing Datasets statistics.}\label{tab:testdata}
%  \end{table}
\subsection{Evaluation Protocols.}

 Evaluation protocols are as follows.

\textbf{GRID}~\cite{grid} contains $250$ probe images and $250$ true match images of the probes in the gallery. Besides, there are a total of $775$ additional images that do not belong to any of the probes. We randomly take out $125$ probe images. The remaining $125$ probe images and $775+250$ images in the gallery are used for testing.

\textbf{i-LIDS}~\cite{ilids} has two versions, images and sequences. The former is used in our experiments. It involves $300$ different pedestrian pairs observed across two disjoint camera views $1$ and $2$ in public open space. We randomly select $60$ pedestrian pairs, two images per pair are randomly selected as probe image and gallery image respectively.

\textbf{PRID2011}~\cite{prid} has single-shot and multi-shot versions. We use the former in our experiments. The single-shot version has two camera views $A$ and $B$, which capture $385$ and $749$ pedestrians respectively. Only $200$ pedestrians appear in both views.  During the evaluation, $100$ randomly identities presented in both views are selected, the remaining $100$ identities in view $A$ constitute probe set and the remaining $649$ identities in view $B$ constitute gallery set.

\textbf{VIPeR}~\cite{viper} contains $632$ pedestrian image pairs. Each pair contains two images of the same individual seen from different cameras $1$ and $2$.  Each image pair was taken from an arbitrary viewpoint under varying illumination conditions. To compare to other methods, we randomly select half of these identities from camera $1$ as probe images and their matched images in $2$ as gallery images.

%For all the testing datasets, the average results over $10$ random splits are reported.
\subsection{Ablation studies on Rotated MNIST.}

\begin{figure*}[h]
    \centering
    \subfigure[]{
      \begin{minipage}[t]{0.45\linewidth}
      \centering
      \includegraphics[scale=1.0]{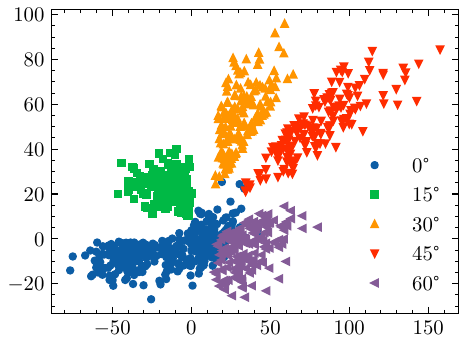}\label{fig:mnist1}
       \end{minipage}}
       \hfill
       \subfigure[]{
       \begin{minipage}[t]{0.45\linewidth}
       \centering
      \includegraphics[scale=1.0]{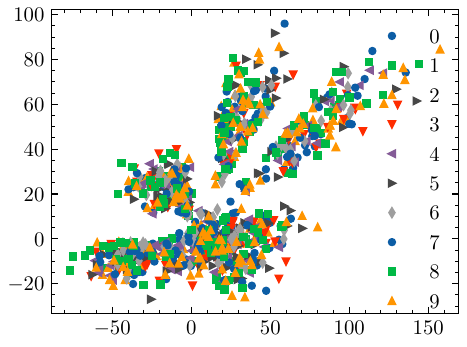}\label{fig:mnist2}
       \end{minipage}}
         \hfill
         \subfigure[]{
         \begin{minipage}[t]{0.45\linewidth}
         \centering
        \includegraphics[scale=1.0]{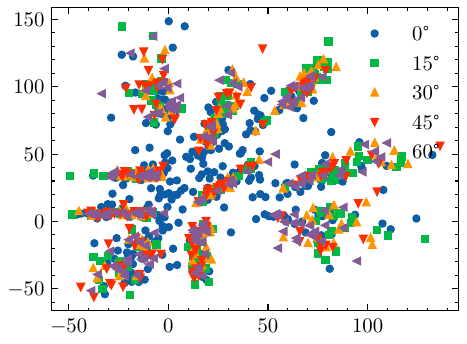}\label{fig:mnist3}
         \end{minipage}}
         \hfill
         \subfigure[]{
          \begin{minipage}[t]{0.45\linewidth}
          \centering
         \includegraphics[scale=1.0]{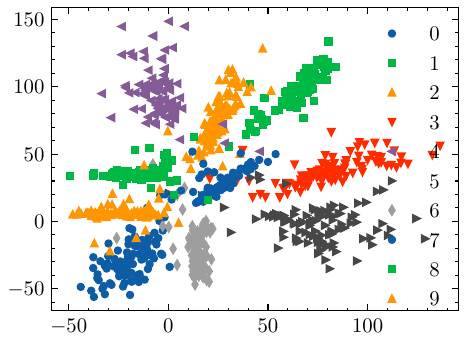}\label{fig:mnist4}
          \end{minipage}}
       \caption{2D embeddings of all two latent subspaces. (a,b): ${v}$ encoded by $f_V$. (c,d): ${s}$ encoded by $f_S$. (a,c) are colored according to their domains and (b,d) are colored according to their classes.}\label{fig:mnist}
 \end{figure*}
\subsubsection{Dataset and Setting}
To verify whether the capability of DIR-ReID model to disentangling $s$ and $v$, we first construct rotated MNIST datasets following~\cite{Ghifary_2015_ICCV}. $100$ images per class ($10$ classes totally) are randomly sampled from the MNIST training dataset, which is denoted by $\mathcal{M}_{0^\circ}$. We then rotated the images in $\mathcal{M}_{0^\circ}$ by $15,30,45$, and $60$ degrees, creating four additional domains. To plot the latent subspaces directly without applying dimensionality reduction, we restrict the size of each latent space to 2 dimensions. In experiments, we train the MDDAN block with an additional reconstruction loss, which is enough to attain a encouraging result. 
\subsubsection{Architecture and Implementation Details}
The architectures of the encoders, classifiers are displayed in Table~\ref{tab:arc_enc}, Table~\ref{tab:arc_cls} respectively. All methods are trained for 500 epochs and the batch size is set to 100. Adam is used to train all the components from scratch with learning rate as 0.001. We also use warmup to linearly increase the learning rate from 0 to 0.001 during the first 100 epochs of training. 

% \begin{table}
%     \centering
%     \begin{tabular}{c|c}
%         \hline \hline 
%         block & details\\ \hline
%         1 &Linear(1024), BatchNormal1d, ReLU\\ 
%         2 & Upsample(2)\\
%         3 & ConvTranspose2d(128,5),BatchNormal2d, ReLU \\
%         4 & Upsample(2)\\
%         5 & ConvTranspose2d(256,5), BatchNormal2d, ReLU\\
%         6 & Conv2d(256, 1)\\\hline \hline 
%     \end{tabular}
%     \caption{Architecture for the generator $G(\mathbf{s}\otimes \mathbf{v})$. The parameter for Linear is output features. The parameters for ConvTranspose2d are output channels and kernel size. The parameter for Upsample is the upsampling factor. The parameters for Conv2d are output channels and kernel size.}\label{tab:arc_gen}
% \end{table}

\begin{table}
    \centering
    \begin{tabular}{c|c}
        \hline \hline 
        block & details\\ \hline
        1 & Conv2d(32, 5), BatchNorm2d, ReLU\\
        2 & MaxPool2d(2, 2)\\
        3 & Conv2d(64, 5), BatchNorm2d, ReLU \\
        4 & MaxPool2d(2, 2)\\
        5 & Linear(2)\\\hline \hline 
    \end{tabular}
    \caption{Architecture for encoders $f_S, f_V$. The parameters for Conv2d are output channels and kernel size. Theparameters for MaxPool2d are kernel size and stride. The parameter for Linear is output features.}\label{tab:arc_enc}
\end{table}

\begin{table}
    \centering
    \begin{tabular}{c|c}
        \hline \hline 
        block & details\\ \hline
        For $\mathcal{C}_V$ &ReLU,Linear($5$ ) \\
        For $\mathcal{C}_S$ &ReLU,Linear($10$) \\ 
        For $\mathcal{C}_C^S$ &ReLU,Linear($5$ ) \\
        For $\mathcal{C}_C^v$ &ReLU,Linear($5$ ) \\\hline \hline 
    \end{tabular}
    \caption{Architecture of classifiers for ID-specific factors, Domain-Specific factors, and
    concatenated vectors. The parameter for Linear is output features.}\label{tab:arc_cls}
\end{table}

\subsubsection{Additional Experimental Results}
 
\begin{table}[]
    \centering
    \begin{tabular}{c|c}
    \hline
    & Test Accuracy on $\mathcal{M}_{75^\circ}$ \\\hline
    Baseline   & $46.4$    \\\hline
    w/ Dual DANN~\cite{ganin2016domain}           & $53.5$      \\
    Improvements$\uparrow$            & $7.1$    \\\hline\hline
    w/  MDDAN           & $58.2$      \\
    Improvements$\uparrow$            & $11.8$    \\\hline
    w/ BA & $61.9$    \\
    Improvements$\uparrow$  & $15.5$   \\\hline\hline
    \end{tabular}
    \caption{Ablation study of three different blocks: dual GRL block, our MDDAN block and the BA block. The reported validation metric is the accuracy of the $\mathcal{M}_{75^\circ}$ dataset. The baseline is only using the encoder $f_S$ and classifier $\mathcal{C}_S$.}
    \label{tab:ablation-mnist}
    \end{table}

    \begin{figure}[h]
        \begin{center}
           \includegraphics[width=1.0\linewidth,scale=1.0]{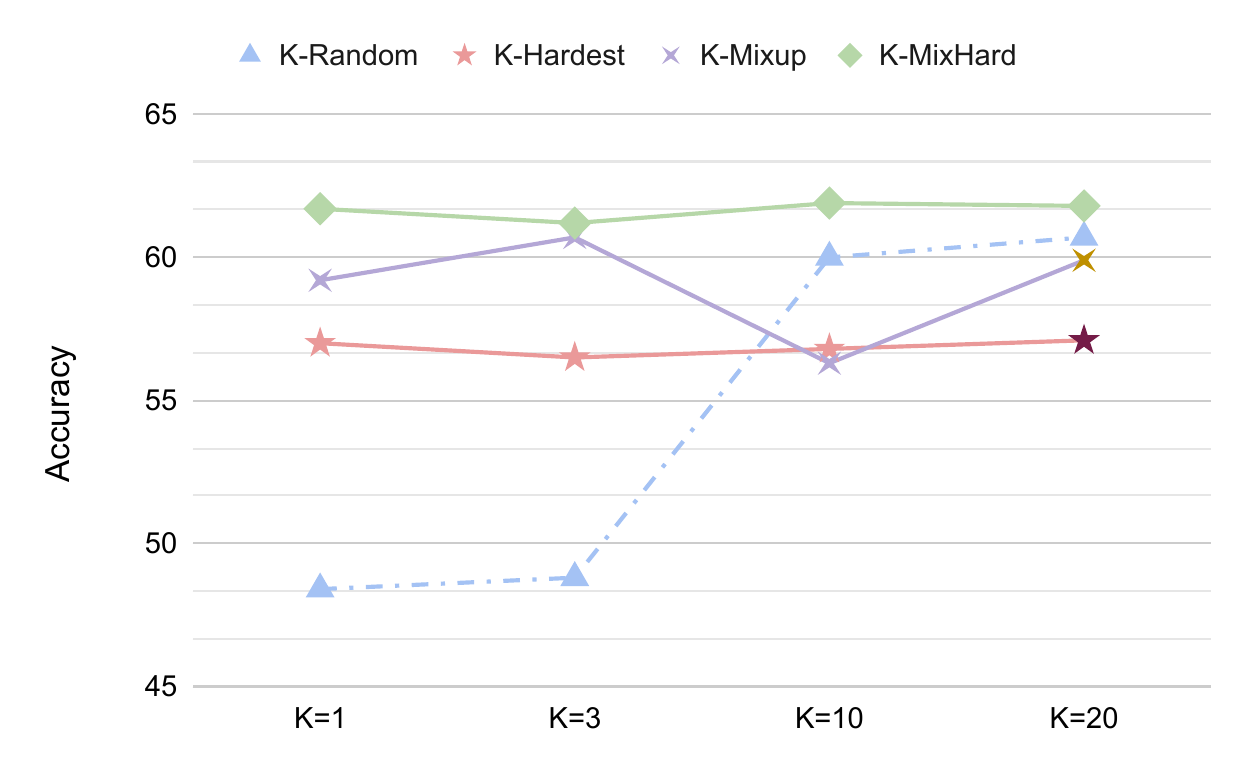}
        \end{center}
           \caption{Ablation study of backdoor adjustment methods. The reported validation metric is the test accuracy of the $\mathcal{M}_{70\circ}$ dataset.}
        \label{fig:ablation-K}
     \end{figure}
\textbf{Analysis of MDDAN.} As shown in Table~\ref{tab:ablation}, directly applying the dual GRL block benefits the generalization ability, while the proposed MDDAN improve the test accuracy on $\mathcal{M}_{75^\circ}$ dataset by a even more large margin, which is $11.8\%$ points.

\textbf{Analysis of methods for backdoor adjustment.} The comparison results are shown in~\figurename~\ref{fig:ablation-K}. Different from BA for Re-ID, here $K$-MixHard attains the most superior performance, which is $61.9\%$ test accuracy. In general, $K-$Random can attain an encouraging performance gain and we can choose other kinds of methods and parameters based on the difficulty of the dataset.

\textbf{Ablation study of different blocks.} By adding the multi-domain disentangled block and the backdoor adjustment block successively, we improve the generalization accuracy from $46.4\%$ to $58.2\%$ and $61.9\%$ respectively (Table~\ref{tab:ablation-mnist}), showing the effectiveness of the proposed model again.

\textbf{Disentanglement on rotated MNIST.} 
% To bring the ability of causal reasoning into DIR-ReID, the most important thing is to distinguish the ID-specific factors. 
The disentanglement results are demonstrated in~\figurename~\ref{fig:mnist}.
We can find a correlation between the rotation angle (domain labels) and ${v}$ in~\figurename~\ref{fig:mnist1}, five domains are clustered into five distinct clusters, while in~\figurename~\ref{fig:mnist2} no clustering is visible, namely there is very weak correlation between $v$ and class labels. By contrast, in~\figurename~\ref{fig:mnist3} no clustering is visible according to the rotation angle. But~\figurename~\ref{fig:mnist4} shows ten distinct clusters, where each cluster corresponds to a class. From these initial qualitative results, we conclude that the dual MDDAN is disentangling the information contained in ${x}$ as intended. ${v}$ only contains domain information and ${s}$ only contains identity information. The great disentangle results ensure the backdoor adjustment can be carried out effectively.

\subsection{Comparision with Similar Adversarial Learning-Based Methods}

Here we discuss similar works DANN~\cite{ganin2016domain}, DDAN~\cite{chen2020dual} and CaNE~\cite{yuan2020calibrated}, which use adversarial training to reduce domain divergence or nuisance divergence. There are three differences: (i) The {\color{red}applications} are different. Given $n$ domains, DANN needs $n$ binary classifiers to check which domain one images belongs to. DDAN selects one central domain, using one binary classifier to check if one image belongs to the central (1) or peripheral (0) domain. CaNE implements adversarial training in nuisance attributes (camera ID and video timestamps). We directly use entropy maximization with multi-domain classification results, which extends the assumption of binary classification in DANN. (ii) The {\color{red}goals} are different. Our DIR-ReID is an algorithmic implementation of backdoor adjustment and adversarial training block (MDDAN) is just one step of our method. We use adversarial training for simultaneously reducing domain divergence and disentangling semantic/variation factors. (iii) We show the underlying {\color{red}optimization objective} of entropy maximization is highly correlated with fusing domain information (Appendix. \ref{app:max_ent}). Secondly, we observe a correlation between MDDAN optimization with mutual information minimization (Appendix. \ref{app:info}).
